# Supplementary material for: Intermittent relaxation and avalanches in extremely persistent active matter
Source: arXiv:2212.09836 ancillary file (2023-06-05)
Supplement: Supplementary file 1 [file add.supp.pdf]

# Supplementary Material to "Intermittent relaxation and avalanches in extremely persistent active matter"

Yann-Edwin Keta,[1] Rituparno Mandal,[2] Peter Sollich,[2, 3] Robert L. Jack,[4, 5] and Ludovic Berthier[1, 4]

[1] *Laboratoire Charles Coulomb (L2C), Université de Montpellier, CNRS, 34095 Montpellier, France*
[2] *Institute for Theoretical Physics, Georg-August-Universität Göttingen, 37077 Göttingen, Germany*
[3] *Department of Mathematics, King's College London, London WC2R 2LS, UK*
[4] *Yusuf Hamied Department of Chemistry, University of Cambridge, Lensfield Road, Cambridge CB2 1EW, United Kingdom*
[5] *Department of Applied Mathematics and Theoretical Physics, University of Cambridge, Wilberforce Road, Cambridge CB3 0WA, United Kingdom*

(Dated: June 5, 2023)

## A. INTERACTION POTENTIAL

We use a regularised inverse power law $1/r^{12}$ pairwise additive potential [1] with

$$U_{ij} = \varepsilon \left[ \frac{1}{(r_{ij}/\tilde{\sigma}_{ij})^a} + c_0 + c_1 (r_{ij}/\tilde{\sigma}_{ij})^2 + c_2 (r_{ij}/\tilde{\sigma}_{ij})^4 \right] \Theta(r_c - r_{ij}/\tilde{\sigma}_{ij}), \tag{A1}$$

$$\tilde{\sigma}_{ij} = \frac{\sigma_i + \sigma_j}{2} (1 - 0.2|\sigma_i - \sigma_j|), \tag{A2}$$

$$a = 12,\ r_c = 1.25,\ c_0 = -\frac{8 + a(a+6)}{8 r_c^a},\ c_1 = \frac{a(a+4)}{4 r_c^{a+2}},\ c_2 = -\frac{a(a+2)}{8 r_c^{a+4}}. \tag{A3}$$

The coefficients $c_0$, $c_1$, and $c_2$ make the potential and its first two derivatives continuous at the cutoff distance $r_c$ – which is needed by the conjugate gradient minimisation method – and the pair interaction is slightly non-additive to improve the glass-forming ability of the system. The continuity of the second derivative of the potential is a necessary condition for the convergence of our conjugate gradient algorithm.

## B. ELASTIC DISPLACEMENTS

We consider the Hessian matrix $\mathbb{H}$ with elements

$$H_{i\gamma,j\delta} = \frac{\partial^2}{\partial r_i^\gamma \partial r_j^\delta} U \tag{B1}$$

where Greek indices are used for spatial dimensions and Latin indices for particles. Eq. (12) is equivalent to

$$-\sum_{j,\delta} H_{i\gamma,j\delta} \delta r_j^\delta + \Xi_{i\gamma} = 0 \tag{B2}$$

and can be inverted as

$$\delta r_{i\gamma} = \sum_{j,\delta} (H^{-1})_{i\gamma,j\delta} \Xi_{j\delta}. \tag{B3}$$

The Hessian matrix $\mathbb{H}$ is symmetric and real-valued so that, by virtue of the spectral theorem, there exists an orthonormal basis of eigenvectors $\boldsymbol{e}_a$, associated with eigenvalues $\Lambda_a$, that diagonalises it:

$$H_{i\gamma,j\delta} = \sum_a \Lambda_a e_{a,i\gamma} e_{a,j\delta}. \tag{B4}$$

Introducing the projection of the affine force along eigenvector $\boldsymbol{e}_a$,

$$\Xi_a = \sum_{j,\delta} \Xi_{j\delta} e_{a,j\delta} \tag{B5}$$

and employing the diagonalised form of the Hessian, Eq. (B3) then becomes

$$\delta r_{i\gamma} = \sum_a \Xi_a \Lambda_a^{-1} e_{a,i\gamma}. \tag{B6}$$

Here we have implicitly omitted eigenvectors with zero eigenvalues $\Lambda_a = 0$: these correspond to translations, which are explicitly excluded from $\delta r_{i\gamma}$ as we work in the centre-of-mass frame.

We now approximate the eigenvectors of $\mathbb{H}$ as the transverse and longitudinal plane wave eigenstates of the Navier operator [2, 3] for the displacement field in an elastic medium, with the associated eigenvalues proportional to the square of the wavevector,

$$a \equiv (m, n, \alpha), \quad \Xi_a \equiv \Xi^\alpha_{mn}, \quad e_{a,i\gamma} \approx e^{\mathrm{i}\boldsymbol{k}_{mn}\cdot\boldsymbol{r}_i} \hat{k}^\alpha_{mn\gamma}/N, \quad \Lambda_a \approx \lambda^\alpha(m^2+n^2)/N \tag{B7}$$

where $\alpha = ||, \perp$ is the polarisation direction, $\boldsymbol{k}_{mn} = (2\pi m/L, 2\pi n/L)$ is the wavevector, $\hat{\boldsymbol{k}}^{||}_{mn} = \boldsymbol{k}_{mn}/|\boldsymbol{k}_{mn}|$, and $\hat{\boldsymbol{k}}^{\perp}_{mn} = \boldsymbol{e}_z \times \hat{\boldsymbol{k}}^{||}_{mn}$. The displacement field (B6) can then be written as

$$\delta r_{i\gamma} = \sum_{m,n,\alpha} \Xi^\alpha_{mn} \frac{e^{\mathrm{i}\boldsymbol{k}_{mn}\cdot\boldsymbol{r}_i} \hat{k}^\alpha_{mn\gamma}}{\lambda^\alpha(m^2+n^2)} \tag{B8}$$

which is equivalent to Eq. (14).

We have checked numerically that the approximate plane wave eigenvectors are still orthonormal to $\mathcal{O}(1/N)$, and that the projections of the affine forces $\boldsymbol{\Xi_i}$ onto both the exact and the approximate eigenvectors of the Hessian $\mathbb{H}$ all have the same variance within statistical accuracy.

## C. RESIDUAL FORCE

We compute the Taylor expansion of the force at time $t$:

$$\begin{aligned} -\nabla U(\boldsymbol{r}(t)) = -\nabla U((\boldsymbol{r}(t)-\boldsymbol{r}(0))+\boldsymbol{r}(0)) &= -\nabla U(\boldsymbol{r}(0)) - \mathbb{H}(0)(\boldsymbol{r}(t)-\boldsymbol{r}(0)) + \mathcal{O}(|\boldsymbol{r}(t)-\boldsymbol{r}(0)|^2) \\ &= -\nabla U(\boldsymbol{r}(0)) + \boldsymbol{f}_{\mathrm{lin}}(t) + \boldsymbol{f}_{\mathrm{res}}(t) \end{aligned} \tag{C1}$$

where $\mathbb{H}(0)$ is the Hessian matrix computed at time 0, $\boldsymbol{f}_{\mathrm{lin}}(t) = -\mathbb{H}(0)(\boldsymbol{r}(t)-\boldsymbol{r}(0))$ is the elastic (linear) force corresponding to the displacement field $\boldsymbol{r}(t)-\boldsymbol{r}(0)$, and $\boldsymbol{f}_{\mathrm{res}}(t)$ is the residual force. The effective potential energy $U_{\mathrm{eff}}$ (7) is minimised at all times, therefore

$$\begin{aligned} & -\nabla U(\boldsymbol{r}(t)) + \boldsymbol{p}(t) - \overline{\boldsymbol{p}(t)} = -\nabla U(\boldsymbol{r}(0)) + \boldsymbol{p}(0) - \overline{\boldsymbol{p}(0)} = 0 \\ \Leftrightarrow\ & \boldsymbol{f}_{\mathrm{res}}(t) = -\boldsymbol{f}_{\mathrm{lin}}(t) - [(\boldsymbol{p}(t)-\overline{\boldsymbol{p}(t)}) - (\boldsymbol{p}(0)-\overline{\boldsymbol{p}(0)})] \\ \Leftrightarrow\ & \boldsymbol{f}_{\mathrm{res}}(t) = \mathbb{H}(0)(\boldsymbol{r}(t)-\boldsymbol{r}(0)) - [(\boldsymbol{p}(t)-\overline{\boldsymbol{p}(t)}) - (\boldsymbol{p}(0)-\overline{\boldsymbol{p}(0)})]. \end{aligned} \tag{C2}$$

One sees that $\boldsymbol{f}_{\mathrm{res}}(t)$ vanishes if and only if the displacement associated with the change in propulsion is purely elastic.

We plot in Fig. C1 the log-distribution of $|\boldsymbol{f}_{\mathrm{res}}(t)|$ for different rescaled times $t' = t/\tau_p$. At intermediate times, the log-distribution is bimodal, with the 2 peaks separated by the value $|\boldsymbol{f}_{\mathrm{res}}| \approx 20$. This is similar to what is observed for supercooled liquids (Ref. [4], Fig. SM4), and we thus use $|\boldsymbol{f}_{\mathrm{res}}| \approx 20$ as the threshold to identify rearranging particles.

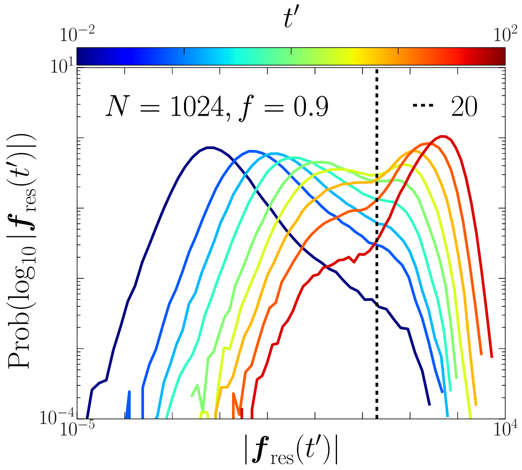


FIG. C1. Log-distribution of residual force (C2) for different lag times $t' = t/\tau_p$.


[1] Ninarello A, Berthier L, Coslovich D. Models and Algorithms for the Next Generation of Glass Transition Studies. Physical Review X. 2017 Jun;7(2):021039.

[2] Slaughter WS. The Linearized Theory of Elasticity. Boston, MA: Birkhäuser Boston; 2002.

[3] Maloney CE. Correlations in the Elastic Response of Dense Random Packings. Physical Review Letters. 2006 Jul;97(3):035503.

[4] Lerbinger M, Barbot A, Vandembroucq D, Patinet S. Relevance of Shear Transformations in the Relaxation of Supercooled Liquids. Phys Rev Lett. 2022 Oct;129:195501. Available from: https://link.aps.org/doi/10.1103/PhysRevLett.129.195501.
